# Supplementary material for: Graph Relation Distillation for Efficient Biomedical Instance Segmentation
Source: arXiv:2401.06370 source file (2024-01-12)
Supplement: Supplementary file 1 [file appendix.tex]

\appendix[Additional Implementation Details]

We use the feed-forward feature tenors after the ReLU layer from each stage of the VGG19 network. We define the patch-wise feature distance in Eq. 1 as
\begin{equation*}
d_f\left(S(p), R(q)\right)=\sum_{i \in N^{L}(p), j \in N^{L}(q)} \frac{C_{S}^{L}\left(i\right) C_{R}^{L}\left(j\right)}{\left\|C_{S}^{L}\left(i\right)\right\|\left\|C_{R}^{L}\left(j \right)\right\|}
\end{equation*}
where $N^{L}(q)$ and $N^{L}(q)$ are the neighboring region of $p$ and $q$ in the $L$-th layer, respectively. $\left\|\cdot\right\|$ denotes the $L_2$ distance. For the neighboring region size, we use $3 \times 3$ for $L = 4, 5$ and $5 \times 5$ for $L = 1, 2, 3$. We use the $L_1$ error to measure the NNF change after each NNF search iteration and set the convergence threshold as 0.001. We set the search radius of the propogation step in NNF searching as 4, 4, 4, 4, 2 from $L=1$ to $L=5$. 

In the deconvolution step (Eq. 2), we set the convergence threshold as 0.001 for the MSE loss function. We use the ADAM optimizer \cite{DBLP:journals/corr/KingmaB14} at a learning rate of 0.05. 

We use 4, 4, 4, 4, 2 (from $L=1$ to $L=5$) as the dilation kernel sizes when obtaining the RoI area from the mask for each layer. We set the checkboard distance threshold for picking near-RoI best buddies as 2, 2, 2, 2, 1 from $L=1$ to $L=5$. These distances are also used as the step-size of each progressive step in the NNF interpolation. In the aggregation function $f(\cdot)$ for the interpolation results around anchors (Eq. 6), we set the upper bound $d_{high}$ as $1/2$ of the width of the RoI area and the lower bound $d_{low}$ as $1/4$ of the width of the RoI area. The nearest-neighbor interpolation is adopted to upsample the NNFs. 

In the two-step warping, we set the local patch size as $3 \times 3$ and thus $n=9$ in Eq. 7. Since the shape of feature from the final layer ($L=1$) is the same as the shape of the image, we operate the matching and interpolation process again on the final layer to obtain more accurate estimations for NNFs and better completed results.

% use section* for acknowledgment
% \section*{Acknowledgment}
